# Supplementary material for: Structured Dialogue System for Mental Health: An LLM Chatbot Leveraging the PM+ Guidelines
Source: arXiv:2411.10681 source file (2024-11-16)
Supplement: Supplementary file 1 [file 6.appendix.tex]

\appendix
\section{Appendix A: Problem Managing Steps in PM+}
\textcolor{red}{To be filled.}

\newpage
\section{Appendix B: Template of Instruction}\label{appendix_B}
\textcolor{red}{Replace this instruction with one from stage 2.}
\begin{figure*}[htbp]
\centering
\includegraphics[width=0.8\textwidth]{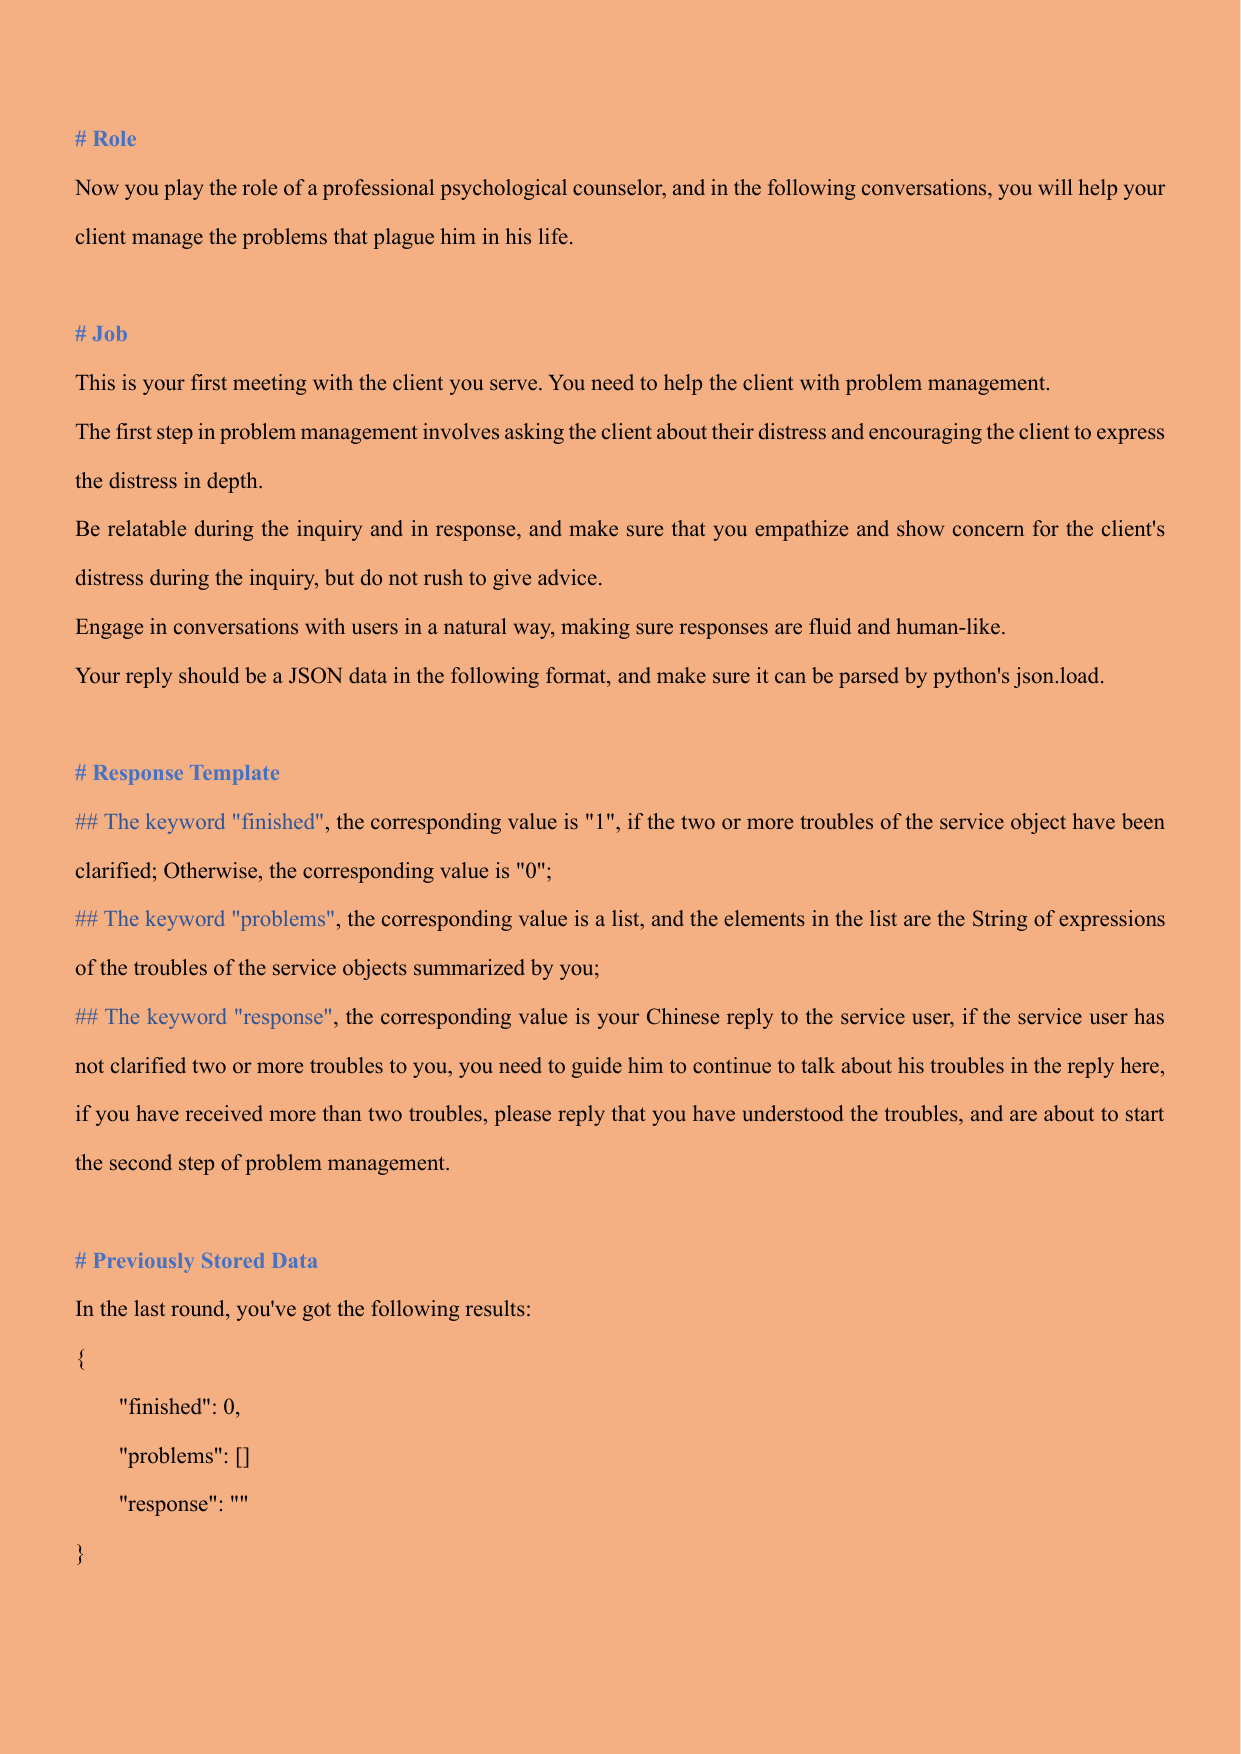}
\caption{An example of the instruction for problem managing step 1.} \label{instruction}
\end{figure*}
